# Supplementary material for: A Methodology for the Offline Evaluation of Recommender Systems in a User Interface with Multiple Carousels
Source: arXiv:2105.06275 source file (2021-05-13)
Supplement: Supplementary file 1 [file appendix.tex]

\appendix

\section{Questions the authors aim to get feedback on during the poster session}

\begin{itemize}
    \item Are the goals of this research sufficiently clear?
    \item Is any related work citation missing? Is the carousel evaluation scenario similar to other scenarios already present in the literature but not cited in the paper?
    \item Is the proposed metric general enough? Which other behaviors should be modeled by the metric?
    % \item Are the experimental findings useful? \nico{Questa non ricordo se la devo togliere}
    \item Considering that an extended offline experimental as well as an online evaluation is included in future work, which kind of scenarios could be useful to explore?
\end{itemize}
